# Supplementary material for: Cluster-induced deagglomeration in dilute gravity-driven gas-solid flows of cohesive grains
Source: arXiv:1804.08074 source file (2018-12-04)
Supplement: Supplementary file 1 [file sm.pdf]

# Cluster-induced Deagglomeration in Dilute Gravity-driven Gas-solid Flows of Cohesive Grains: Supplemental Materials

Peiyuan Liu and Christine M. Hrenya*
*Department of Chemical and Biological Engineering,*
*University of Colorado Boulder, Boulder, Colorado, 80309, USA*
(Dated: December 3, 2018)

In Supplemental Materials, we provide data on time evolution of flow properties under different domain size and cohesion levels. In addition, the flow properties under independent variation of bed width and height, as well as the variation of superficial gas velocity, are discussed. Finally, detailed derivation on the singlet-doublet collisional cross section is included.

* Corresponding author: hrenya@colorado.edu

## I. TIME EVOLUTION OF FLOW PROPERTIES

The time evolution of the flow properties, including the mean particle streamwise ($y$-direction) velocity $\bar{v}_y$, heterogeneity index $D$ and fraction of particles in agglomerates $A$, is provided in Fig. S1 and S2, which show the evolution with increasing system size ($W$) and cohesion level (Bo $= F_c/mg$, where $m$ is the mass of a single grain and $F_c$ is the magnitude of cohesive force varying from 340 nN to 2720 nN), respectively. As time evolves, all three flow properties level off and fluctuate around their corresponding time-averaged values over a duration of 1–4 s (shaded areas), indicating the existence of statistical state states. Corresponding movies of the flow patterns transitioning from initial states to steady states (0–1 s) are uploaded as "`Flow_evolutions_increasing_domain_size.mp4`" and "`Flow_evolutions_increasing_cohesion.mp4`". In the main paper, we focus on the time-averaged flow properties collected within 1–4 s (marked by horizontal dashed lines on Fig. S1 and S2), when all systems studied in this work have reached their corresponding statistical steady states.

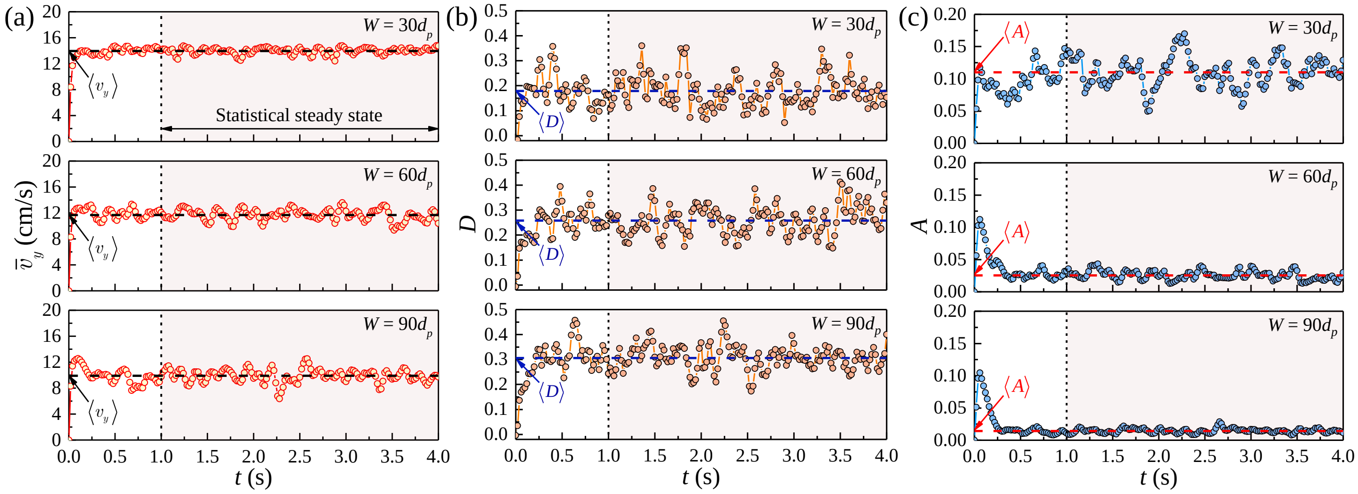


FIG. S1. Time evolutions of (a) mean particle streamwise ($y$-direction) velocity $\bar{v}_y$, (b) heterogeneity index $D$ and (c) fraction of particles in agglomerates $A$ with increasing system size $W$ ($H = 4W$) at a fixed granular bond number Bo $= F_c/mg = 161$. Horizontal dashed lines mark the corresponding time-averaged values for each time evolution over the statistical steady state from $t = 1$ s to 4 s (shaded).

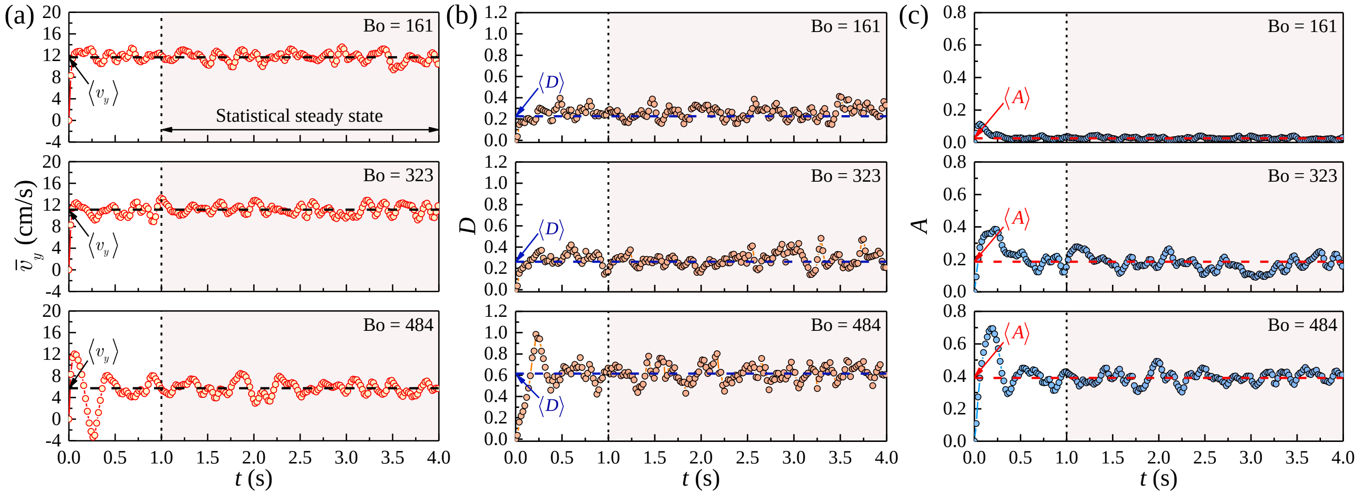


FIG. S2. Time evolutions of (a) mean particle streamwise ($y$-direction) velocity $\bar{v}_y$, (b) heterogeneity index $D$ and (c) fraction of particles in agglomerates $A$ with increasing granular bond number Bo $= F_c/mg$ (where $F_c$ varies from 340 nN to 2720 nN) at a fixed system size $W = 60d_p$ ($H = 240d_p$). Horizontal dashed lines mark the corresponding time-averaged values for each time evolution over the statistical steady state from $t = 1$ s to 4 s (shaded).

## II. FLOW PROPERTIES UNDER INDEPENDENT VARIATION OF BED WIDTH AND HEIGHT

We check the sensitivity of system properties (agglomeration fraction $\langle A\rangle$, heterogeneity index $\langle D\rangle$ and granular temperatures $\langle T_i\rangle$) to increasing bed width $W$ and height $H$ individually (without keeping a constant aspect ratio) via simulations. The results are summarized in Fig. S3, where it can be seen that: i. Increasing $W$ while fixing $H$ ("walking along the $x$-$z$-plane" only) leads to pronounced change of $\langle A\rangle$, $\langle D\rangle$ and $\langle T_i\rangle$ (Fig. S3a-c); ii. Increasing $H$ while fixing $W$ ("walking along the $y$-direction" only) has little impact on $\langle A\rangle$, $\langle D\rangle$ and $\langle T_i\rangle$ (Fig. S3d-f), except for an initial larger sensitivity as $H$ increases from $120d_p$ to $240d_p$; and when $H \geq 240d_p$ ($H/W \geq 4$), all system properties level off, similar to the finding on the gas-solid flows of non-cohesive particles [1].

Both observations are associated with the system anisotropy, where mean flows with stronger inertia act along the $y$-direction only. Thus, $W$ serves as the characteristic length in the mean-flow Reynolds number ($\mathrm{Re}_g = |U - \langle v_y\rangle|\,\rho_g W/\mu_g$, where $U$ is superficial gas velocity and $\langle v_y\rangle$ is mean particle streamwise velocity in steady states) and plays a leading role in determining system properties.

In single-phase pipe flows, increasing pipe diameter enhances hydrodynamic instabilities (turbulence). Analogously, in gas-solid systems considered in current work, extending $W$ (while fixing $H$) leads to more clustering instabilities of the solid phase so that the heterogeneity index $\langle D\rangle$ grows with $W$ (Fig. S3b). Larger clusters tend to fall and collide with individual particles/smaller clusters flowing upwards, causing an increase in granular temperatures $\langle T_i\rangle$ (Fig. S3c). The increased velocity fluctuations at higher $\langle T_i\rangle$ contribute to effective separation of particles in agglomerates, reducing $\langle A\rangle$ and $\langle a\rangle$ with $W$ (Fig. S3a), so that the "cluster-induced deagglomeration" mechanism remains robust.

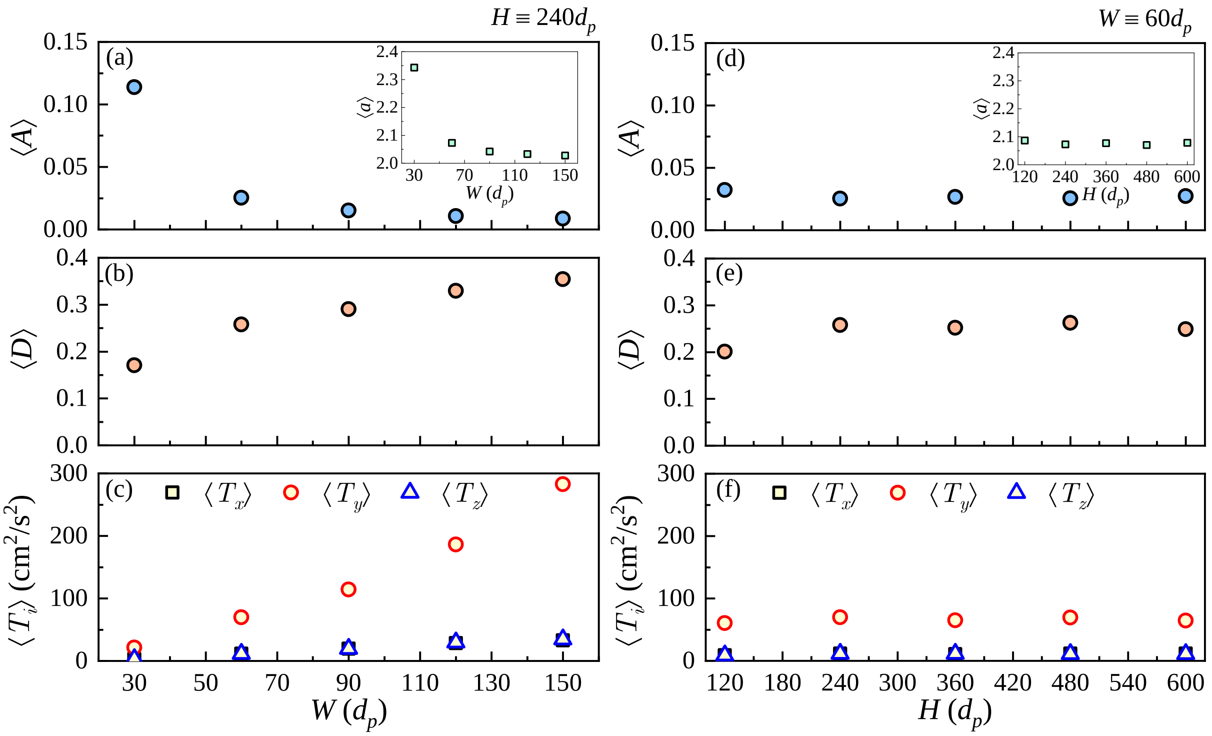


FIG. S3. Steady-state (a) agglomerate fraction $\langle A\rangle$, (b) heterogeneity index $\langle D\rangle$ and (c) granular temperatures $\langle T_i\rangle$ as a function of domain width $W$ under a fixed domain height $H \equiv 240d_p$; (d) $\langle A\rangle$, (e) $\langle D\rangle$ and (f) $\langle T_i\rangle$ as a function of $H$ under a fixed $W \equiv 60d_p$. Insets on (a) and (d): steady-state mean agglomerate size $\langle a\rangle$ with increasing $W$ and $H$, respectively.

## III. FLOW PROPERTIES UNDER THE VARIATION OF SUPERFICIAL GAS VELOCITY

Fig. S4 summarizes the results of simulations varying the superficial gas velocity $U$ from 21.5 cm/s to 107.5 cm/s. It can be seen that all system properties are insensitive to $U$, except for the mean particle velocity in the streamwise direction $\langle v_y\rangle$ (Fig. S4d), which increases linearly with $U$. A physical understanding of the observation is detailed below.

During statistical steady states of the unbounded fluidization considered here, particles approximately maintain their terminal velocities ($\sim \langle v_y \rangle$) with their gravity balanced by the gas-solid interaction (that scales with mean gas-solid streamwise slip velocity $U - \langle v_y \rangle$). Since the total weight of the particles is fixed, increasing $U$ does not affect the gas-solid interaction in steady states (where $U - \langle v_y \rangle$ remains flat with increasing $U$ in Fig. S4e, as well as the mean-flow Reynolds number $\mathrm{Re}_g = |U - \langle v_y \rangle| \rho_g W / \mu_g$ and particle Reynolds number $\mathrm{Re}_p = |U - \langle v_y \rangle| \rho_g d_p / \mu_g$), which leaves $\langle D \rangle$, $\langle A \rangle$, $\langle a \rangle$ and $\langle T_i \rangle$ insensitive to $U$ (Fig. S4a–c).

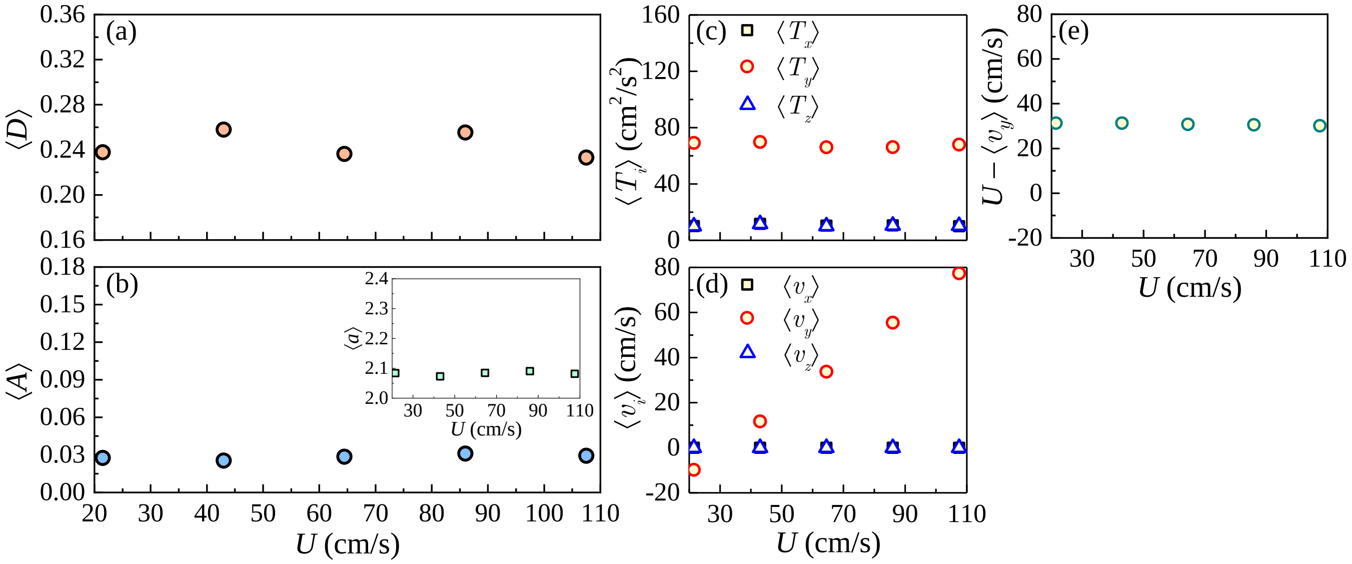


FIG. S4. Steady-state (a) heterogeneity index $\langle D \rangle$, (b) agglomerate fraction $\langle A \rangle$, (c) granular temperatures $\langle T_i \rangle$, (d) particle velocities $\langle v_i \rangle$ and (e) mean gas-solid streamwise slip velocity $U - \langle v_y \rangle$ as a function of superficial gas velocity $U$ under a fixed domain size with $W = 60d_p$, $H = 240d_p$. Insets on (b): steady-state mean agglomerate size $\langle a \rangle$ with increasing $U$.

## IV. COLLISIONAL CROSS SECTION FOR SINGLET-DOUBLET COLLISIONS

For single-doublet collisions, the collisional cross section $s_{12}$, defined as the area that the center of the singlet must lie in to collide with the doublet, is dependent on the orientation angle of doublets. The orientation angle of doublets $\phi$ is defined as the angle between the line connecting the centers of two particles in the doublet and an arbitrary reference plane. As illustrated in Fig. S5a, selecting $x$-$z$ plane (the plane normal to the streamwise direction) as the reference plane, $\phi$ varies from 0 to $\pi/2$, rotating the doublet from "horizontal" to "vertical" orientations (see the detected doublets with color contoured by $\phi$ in a box from the simulation with $W = 60d_p$, $H = 240d_p$ and Bo $= 161$). Collecting values of $\phi$ for the doublets detected in our systems during statistical steady states, we found the distribution functions of $\phi$ with increasing system size follow the $f(\phi) = \cos\phi$, as demonstrated in Fig. S6, where a higher frequency is seen for doublets with smaller $\phi$ (i.e. more doublets with relatively horizontal than vertical orientations). A physical understanding of the higher frequency at smaller $\phi$ is as follows: since the granular temperatures in the two horizontal (transverse, $x$- and $z$-) directions are lower than the vertical (streamwise, $y$-) direction (see Fig. 3b in the main paper, where $T_x$ and $T_z$ are smaller than $T_y$), a pair of particles lining up more horizontally before colliding are more likely to have smaller normal collisional impact velocity, which results in a higher probability of agglomeration and thus more horizontal doublets with smaller $\phi$ collected.

With the distribution of $\phi$ known, we take the dependency of $s_{12}$ on $\phi$ into account in Eq. (1) of the main paper by using the average singlet-doublet collisional cross section weighted over different orientation angles, such that

$$s_{12} = \int_0^{\frac{\pi}{2}} s_{12}(\phi) \cos\phi d\phi. \tag{S1}$$

Based on geometrical considerations, the singlet-doublet collisional cross section as a function of doublet orientation angle $s_{12}(\phi)$ (an example shown as the shaded area on Fig. S5b) is given by

$$s_{12}(\phi) = \frac{1}{2} d_p^2 \left[ \cos\phi \sqrt{4 - \cos^2\phi} - 4 \arccos\left( \frac{1}{2} \cos\phi \right) + 4\pi \right]. \tag{S2}$$

Plugging Eq. (S2) to Eq. (S1) and numerically evaluating the integral gives $s_{12} = 4.66d_p^2$, which is used in Eq. (1) of the main paper.

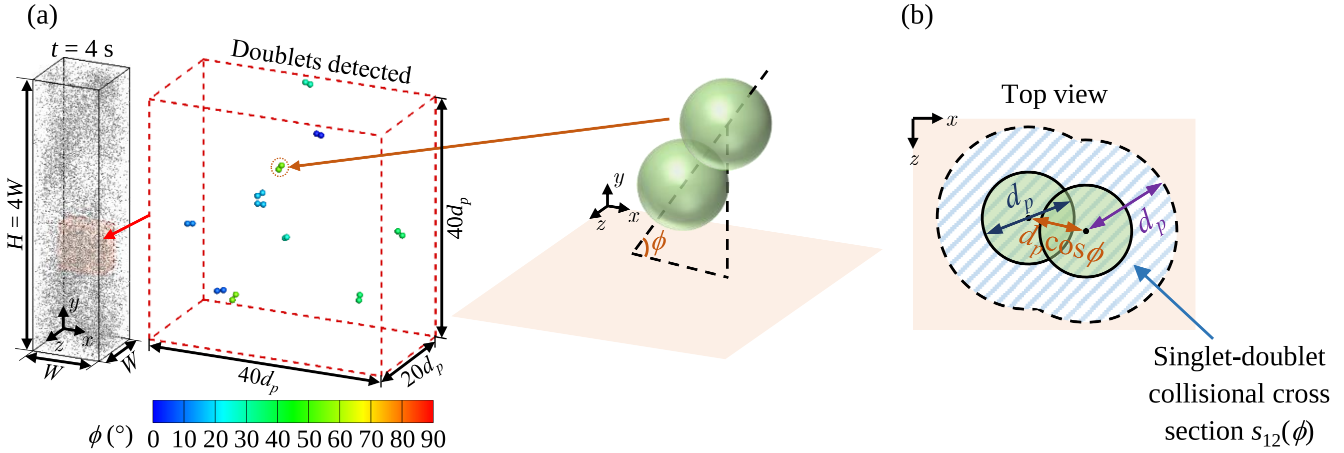


FIG. S5. (a) Isolation of one doublet from the snapshots of particles at $t = 4$ s in the simulation with $W = 60d_p$ ($H = 240d_p$ and Bo = 161). The doublet orientation angle $\phi$, defined as the angle between the line connecting the centers of two particles in the doublet and the $x$-$z$ plane, is marked on the view of the isolated doublet. (b) Projection of the isolated doublet on the $x$-$z$ plane with the corresponding singlet-doublet collisional cross section filled by the shaded area.

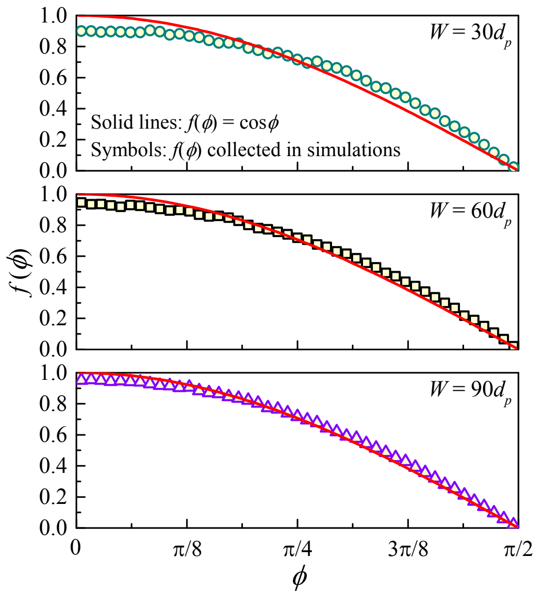


FIG. S6. Distributions of doublet orientation angle $\phi$ collected in statistical steady states with increasing system size (symbols). The distribution functions at all system sizes are well described by $f(\phi) = \cos\phi$ (solid lines).

[1] K. Agrawal, P. N. Loezos, M. Syamlal, and S. Sundaresan, J. Fluid Mech. **445**, 151 (2001).
